# Supplementary material for: Overcoming Catastrophic Forgetting in Graph Neural Networks with Experience Replay
Source: arXiv:2003.09908 source file (2021-02-08)
Supplement: Supplementary file 1 [file Appendix.tex]

\subsection{Derivations of Eq.(\ref{derivation})}
Without loss of generality, we assume the model $f_{\bm{\theta}}$ is  parameterized by $\bm{\theta}$ and the number of training examples is $N$. As is often the case, we obtain the optimal parameters by training our model on the training set:
\begin{equation}
\label{appendix1}
\bm{\theta}=\arg \min _{\bm{\theta} \in \Theta}(\frac{1}{N} \sum_{i=1}^{N} \mathcal{L}(\bm{\theta}, v_{i})),
\end{equation}
where $v_{i}$ is the $i$-th training sample, and $\mathcal{L}$ denotes the loss function. We can remove one training example $v_{\star}$ from the training set.
% and obtain a new training set. 
Then we can compute the change of optimal parameters if $v_{\star}$ was upweighted by some small $\epsilon$, which gives the new parameters:
\begin{equation}
\label{appendix2}
\bm{\theta_{\epsilon,\star}} \stackrel{\text{def}}{=} \arg \min _{\bm{\theta} \in \Theta}(\frac{1}{N} \sum_{i=1}^{N} \mathcal{L}(\bm{\theta}, v_{i})+\epsilon \mathcal{L}(\bm{\theta}, v_{\star})).
\end{equation}
For clarity, we define $R(\bm{\theta}) \stackrel{\text{def}}{=} \frac{1}{N} \sum_{i=1}^{N} \mathcal{L}(\bm{\theta}, v_{i})$. Therefore Eq~\ref{appendix2} can be rewritten as:
\begin{equation}
\label{appendix3}
\bm{\theta_{\epsilon,\star}} \stackrel{\text{def}}{=} \arg \min _{\bm{\theta} \in \Theta}(R(\bm{\theta}) + \epsilon \mathcal{L}(\bm{\theta}, v_{\star})).
\end{equation}
Here loss function $\mathcal{L}$ is convex by assumption, and $\bm{\theta_{\epsilon,\star}}$ can be derived by first-order derivative:
\begin{equation}
\nabla R(\bm{\theta_{\epsilon, \star}})+\epsilon \nabla \mathcal{L}(\bm{\theta_{\epsilon, \star}}, v_{\star})=0.
\end{equation}
Based on the Taylor expansion, we can obtain:
\begin{align}
\label{appendix4}
\nabla R(\bm{\theta_{\epsilon, \star}}) &+\epsilon \nabla \mathcal{L}(\bm{\theta_{\epsilon, \star}}, v_{\star}) \approx \nabla R(\bm{\theta})+\epsilon \nabla \mathcal{L}(\bm{\theta}, v_{\star}) +  \notag
\\ & \left[\nabla^{2} R(\bm{\theta})+\epsilon \nabla^{2} \mathcal{L}(\bm{\theta}, v_{\star})\right](\bm{\theta_{\epsilon,\star}}-\bm{\theta}).
\end{align}
Since $\bm{\theta}$ minimize the convex loss function $R(\bm{\theta}) = \frac{1}{N} \sum_{i=1}^{N} \mathcal{L}(\bm{\theta_{\epsilon,\star}}, v_{i})$, we can get $\nabla R(\bm{\theta}) = 0$ and rewrite Eq~\ref{appendix4} as:
\begin{align}
\label{appendix5}
\bm{\theta_{\epsilon,\star}}-\bm{\theta} = & - \left[\nabla^{2} R(\bm{\theta})+\epsilon \nabla^{2} \mathcal{L}(\bm{\theta}, v_{\star})\right]^{-1} \notag
\\ & \left[\nabla R(\bm{\theta}) + \epsilon \nabla \mathcal{L}(\bm{\theta}, v_{\star}) \right].
\end{align}
In addition, $\epsilon$ is very small which means we have:
\begin{align}
\label{appendix6}
\bm{\theta_{\epsilon,\star}}-\bm{\theta} \approx -\nabla^{2} R(\bm{\theta})^{-1} \nabla \mathcal{L}(\bm{\theta}, v_{\star}) \epsilon.
\end{align}
Now, we can calculate the change of parameters when the weight of the training sample changes:
\begin{align}
\label{appendix7}
\frac{\partial \bm{\theta_{\epsilon,\star}}}{\partial \epsilon}= -\nabla^{2} R(\bm{\theta})^{-1} \nabla \mathcal{L}(\bm{\theta}, v_{\star}).
\end{align}
where $\nabla^{2} R(\bm{\theta})$ is the Hessian matrix: 
\begin{equation}
\label{appendix8}
\mathbf{H}_{\bm{\theta}} \stackrel{\text { def }}{=} \nabla^{2} R(\bm{\theta}) = \frac{1}{N} \sum_{i=1}^{N} \nabla_{\bm{\theta}}^{2} \mathcal{L}(\bm{\theta}, v_{i}),
\end{equation}
and Eq~\ref{appendix7} can be rewritten as:
\begin{align}
\label{appendix9}
\frac{\partial \bm{\theta_{\epsilon,\star}}}{\partial \epsilon}= - \mathbf{H}_{\bm{\theta}}^{-1} \nabla \mathcal{L}(\bm{\theta}, v_{\star}).
\end{align}

\subsection{Details of Experiments}

\subsubsection{Dataset details:} Three benchmarks in our evaluation consist of two citation networks (Cora and Citeseer) and a social network (Reddit). (i) The Cora dataset contains 2,708 machine learning publications grouped into seven classes. (ii) The Citeseer dataset contains 3,327 scientific papers grouped into six categories. Each paper in Cora and Citeseer is represented by a one-hot vector indicating a word's presence or absence from a dictionary. (iii) The Reddit dataset is an undirected graph formed by posts collected from the Reddit discussion forum. Two posts are linked if they contain comments by the same user. Each post has a label indicating the community to which it belongs.

\subsubsection{Hyperparameter setting:} We list the hyperparameters of the three instances of our framework ER-GNN (i.e., ER-GAT, ER-SGC, and ER-GIN) in Table~\ref{ER_GAT}, ~\ref{ER_SGC}, ~\ref{ER_GIN}, respectively.  Note that: (i) Alpha in LeakyRelu is the slope of the negative x-axis. (ii) The number of attention heads is 2 since GAT employs a multi-head attention mechanism to stabilize self-attention learning.

\begin{table}[htbp]
	\centering
	\begin{tabular}{c|c}
		\bottomrule
		\textbf{Hyperparameter} & \textbf{Value} \\
        \hline
        embedding dimensionality & 8\\
        \hline
        epochs & 800\\
        \hline
        learning rate & 0.005\\
        \hline
        decay factor & $5 * 10 ^{-4}$\\
        \hline
        alpha in LeakyRelu & 0.2\\
        \hline
        dropout & 0.4\\
        \hline
        number of attention heads & 2\\
		\toprule
	\end{tabular}
	\caption{The hyperparameters in ER-GAT.}
	\label{ER_GAT}
\end{table}
\begin{table}[htbp]
	\centering
	\begin{tabular}{c|c}
		\bottomrule
		\textbf{Hyperparameter} & \textbf{Value} \\
        \hline
        embedding dimensionality & 16\\
        \hline
        epochs & 100\\
        \hline
        learning rate & 0.2\\
        \hline
        decay factor & $5 \times 10 ^{-6}$\\
		\toprule
	\end{tabular}
	\caption{The hyperparameters in ER-SGC.}
	\label{ER_SGC}
\end{table}

\begin{table}[htbp]
	\centering
	\begin{tabular}{c|c}
		\bottomrule
		\textbf{Hyperparameter} & \textbf{Value} \\
        \hline
        embedding dimensionality & 8\\
        \hline
        epochs & 1000\\
        \hline
        learning rate & 0.001\\
        \hline
        decay factor & $5 \times 10 ^{-6}$\\
		\toprule
	\end{tabular}
	\caption{The hyperparameters in ER-GIN.}
	\label{ER_GIN}
\end{table}
